# Supplementary material for: CLIP the Gap: A Single Domain Generalization Approach for Object Detection
Source: arXiv:2301.05499 source file (2023-03-06)
Supplement: Supplementary file 1 [file supp.tex]

\section{Prompt Curation}

As mentioned in our main paper, we curate a set of domain prompts $\mathcal{P}^t$. For this step, we get the words matching the concept \emph{weather} from WordNet~\cite{wordnet}.~\cref{tab:hyponyms} lists the hyponyms for the word \emph{weather}. With this list, we filter out words that have cosine distance below $0.5$ w.r.t the \emph{weather} in CLIP embedding space. We further improve our wordlist using GloVE~\cite{pennington2014glove} to weed out the uncommon words. To this end, we take only the words which are in the 10k most common words of GloVE.~\cref{tab:glove_prune} lists the words after this stage. 

\begin{table}[h]
    \centering
    \begin{tabular}{|c|}
    \hline
        draft , easter , elements , depression , wave , quiet , snow ,\\ sunshine , fog , blast , freeze , breath , wind , atmosphere ,\\ rainfall , warming , trade , blow , calm , cyclone , rain , air , low , high\\
        \hline
    \end{tabular}
    \caption{Word list after CLIP and GloVE~\cite{pennington2014glove} based pruning}
    \label{tab:glove_prune}
\end{table}

We still see there are words that show the same concepts like \emph{draft , easter , elements , depression , air , low , high, wind, atmosphere, air}  represent related to the windy or stormy conditions, hence we replace these words with \emph{stormy}. We merge \emph{rainfall} and \emph{rain}, while removing ambiguous words like \emph{blast,warming,breath,quiet}.

\begin{table*}[t]
    \centering
    \begin{tabular}{|l|}
    \hline
    scattering , current of air , draft , norther , line storm , doldrums , flurry \\
 
roughness , sou'wester , shower , gale , simoon , trade wind , boisterousness \\
 
deluge , air mass , southerly , easter , west wind , mizzle , whiff \\
 
cold wave , downfall , murk , line squall , elements , bad weather , easterly \\
 
sprinkling , balminess , depression , monsoon , cloudburst , chinook wind , good weather \\
 
fine spray , harmattan , clemency , tramontane , south wind , gentle breeze , wave \\
 
tramontana , draught , windlessness , equinoctial storm , fohn , overcast , cloud cover \\
 
quiet , moderate breeze , souther , thundershower , foehn , westerly , stillness \\
 
airstream , north wind , whiteout , snow eater , levanter , catabatic wind , clear-air turbulence \\
 
fair weather , snow , antitrades , simoom , bize , windiness , fresh gale \\
 
drizzle , sunshine , fog , puff of air , bluster , heat wave , light air \\ 
 
blast , zephyr , whole gale , temperateness , thawing , calmness , squall \\ 
 
storminess , prevailing westerly , soaker , snowfall , hot weather , scorcher , fresh breeze \\
 
raw weather , puff , rough water , northwest wind , murkiness , cold weather , gentle wind \\
 
northwester , freeze , crosswind , gust , mildness , breath , near gale \\
 
east wind , wind , northerly , rainstorm , chinook , atmosphere , rain shower \\
 
rainfall , high wind , pelter , snow flurry , southeaster , virga , jet stream \\
 
breeze , softness , warming , khamsin , atmospheric state , downpour , downdraft \\
 
cloudiness , trade , blow , inclementness , antitrade , strong gale , antitrade wind \\
 
calm , light breeze , tempestuousness , wester , lull , thaw , choppiness \\
  
cyclone , calm air , sleet , sandblast , sea breeze , mistral , air current \\
 
hail , southwester , rain , waterspout , sultriness , katabatic wind , torrent \\ 
 
precipitation , headwind , moderate gale , boreas , breeziness , tailwind , air \\ 
 
sou'easter , low , anticyclone , samiel , thermal , strong breeze , Santa Ana \\ 
 
bise , frost , high , sprinkle , inclemency , turbulence , fogginess  \\
    \hline
    \end{tabular}
    \caption{Hyponyms of word \emph{weather} in WordNet~\cite{wordnet}}
    \label{tab:hyponyms}
\end{table*}
